# Supplementary material for: Optimal electro-mechanical control of the excitonic fine structures of droplet epitaxial quantum dots
Source: arXiv:1803.00340 source file (2018-08-31)
Supplement: Supplementary file 1 [file Biaxial_supple_pr.pdf]

# Supplementary information for "Optimal electro-mechanical control of the excitonic fine structures of droplet epitaxial quantum dots"

Shun-Jen Cheng, Yi Yang, Yu-Nien Wu, Yu-Huai Liao, and Guan-Hao Peng

*Department of Electrophysics, National Chiao Tung University,*

*Hsinchu 30050, Taiwan, Republic of China.*

## S1. GROUP THEORY ANALYSIS FOR EXCITON FINE STRUCTURES OF GAAS QUANTUM DOTS

### A. Bulk of $T_d$ symmetry

The lattice structure of GaAs belongs to $T_d$ symmetry. Table S1 shows the character table for the spin double group $T_d$. In Table S1, $\Gamma_1, \Gamma_2, ...\Gamma_5$ are the irreducible representations (irreps.) of the group $T_d$, and $\Gamma_6, \Gamma_7$ and $\Gamma_8$ are the extra irreps. of the double group $T_d$. The conduction band of GaAs belongs to the scalar irrep. $\Gamma_{1c}$, the valence band belongs to the vector irrep. $\Gamma_{5v}$, and the spin belongs to the doublet irrep. $\Gamma_{6s}$. In this note, the subscript indices $c$, $v$, $X$ and $s$ will be used to indicate conduct band, valence band, exciton state and spin, respectively.

Considering the intrinsic spin-orbit interaction (SOI) in the $T_d$ crystal, we make the product of the conduction band and the spin states, $\Gamma_{1c} \times \Gamma_{6s} = \Gamma_{6c}$, which is a doublet irrep. For the valence states, the SOI makes the valence band split into a doublet and a four-fold band, $\Gamma_{5v} \times \Gamma_{6s} = \Gamma_{7v} + \Gamma_{8v}$, where $\Gamma_{8v}$ is the topmost four-fold valence band, composed of the heavy-hole (HH) and light-hole (LH) bands directly relevant to the exciton under our study. The states of the exciton bound by electron-hole Coulomb interaction in a $T_d$ crystal are created from the direct product of the conduction band and the valence band, $\Gamma_{6c} \times \Gamma_{8v} = \Gamma_{3X} + \Gamma_{4X} + \Gamma_{5X}$, which consists of a doublet $\Gamma_{3X}$ and two triplets $\Gamma_{4X}$, $\Gamma_{5X}$.

To determine the optical activation of exciton, we derive the polarization selection rule

TABLE S1: **The character table of the spin double group $T_d$.**

| $T_d$ | $E$ | $8C_3$ | $3C_2$ | $6S_4$ | $6\sigma_d$ |
|---|---|---|---|---|---|
| $\Gamma_1$ | 1 | 1 | 1 | 1 | 1 |
| $\Gamma_2$ | 1 | 1 | 1 | $-1$ | $-1$ |
| $\Gamma_3$ | 2 | $-1$ | 2 | 0 | 0 |
| $\Gamma_4$ | 3 | 0 | $-1$ | 1 | $-1$ |
| $\Gamma_5$ | 3 | 0 | $-1$ | $-1$ | 1 |
| $\Gamma_6$ | 2 | 1 | 0 | $\sqrt{2}$ | 0 |
| $\Gamma_7$ | 2 | 1 | 0 | $-\sqrt{2}$ | 0 |
| $\Gamma_8$ | 4 | $-1$ | 0 | 0 | 0 |

TABLE S2: **The character table of the spin double group $C_{2v}$.**

| $C_{2v}$ | $E$ | $C_{2z}$ | $\sigma_y$ | $\sigma_x$ | Basis function |
|---|---|---|---|---|---|
| $\Gamma_1$ | 1 | 1 | 1 | 1 | $z$ |
| $\Gamma_2$ | 1 | −1 | 1 | −1 | $x$ |
| $\Gamma_3$ | 1 | 1 | −1 | −1 | $xy$ |
| $\Gamma_4$ | 1 | −1 | −1 | 1 | $y$ |
| $\Gamma_5$ | 2 | 0 | 0 | 0 | |

following the Wigner-Eckart theorem. In the group $T_d$, a photon belongs to the vector irrep. $\Gamma_5$ and the "vacuum state" with no exciton belongs to $\Gamma_1$ (i.e. perfect symmetry). The direct products of the irreps. for photon and exciton can be expressed as below:

$$\Gamma_1 \notin \Gamma_5 \times \Gamma_{3X} = \Gamma_4 + \Gamma_5, \tag{1}$$

$$\Gamma_1 \notin \Gamma_5 \times \Gamma_{4X} = \Gamma_2 + \Gamma_3 + \Gamma_4 + \Gamma_5, \tag{2}$$

$$\Gamma_1 \in \Gamma_5 \times \Gamma_{5X} = \Gamma_1 + \Gamma_3 + \Gamma_4 + \Gamma_5. \tag{3}$$

Equation (3) shows that $\langle\Gamma_1|\,\Gamma_5\,|\Gamma_{5X}\rangle \neq 0$ and, according to the Wigner-Eckart theorem, implies that the exciton in the triplet irrep. $\Gamma_{5X}$ (the triple-degenerate state) is optically active (bright exciton). On the other hand, the other two in the irreps. $\Gamma_4$ and $\Gamma_3$ are shown optically inactive (dark exciton).

## B. Quantum dots in the $C_{2v}$ symmetry

Next, we consider elongated QDs in the shape of $C_{2v}$ symmetry made of host material of $T_d$ symmetry such as GaAs. Table S2 presents the character table for the group $C_{2v}$ with $\Gamma_5$ being the irrep. of the double group of $C_{2v}$. In the last column of the table, the basis functions for each irrep. are listed, according to which the polarizations of the emitted photons can be determined.

With the $C_{2v}$ quantum confinement, the conduction band remains to be in the scalar irrep. $\Gamma_{1c}$, while the valence band is reduced to three singlet ones, $\Gamma_{5v}^{(T_d)} = \Gamma_{1v} + \Gamma_{2v} + \Gamma_{4v}$, where $\Gamma_{2v}$ and $\Gamma_{4v}$ represent the topmost valence bands directly relevant to exciton under our study. In the group $C_{2v}$, the spin belongs to the doublet irrep. $\Gamma_{6s}^{(T_d)} = \Gamma_{5s}$. Again, including the effect of SOI, the conduction band turns out to be a doublet irrep. $\Gamma_{1c} \times \Gamma_{5s} = \Gamma_{5c}$

denoted by $|\uparrow_e\rangle$, $|\downarrow_e\rangle$, and the topmost valence bands $\Gamma_{2v}$ and $\Gamma_{4v}$ split into two doublet irreps. $\Gamma_{2v} \times \Gamma_{5s} = \Gamma_{5v}^{(2)}$ denoted by $|\Uparrow_h\rangle$, $|\Downarrow_h\rangle$ (referred to as the doublet HH bands) and $\Gamma_{4v} \times \Gamma_{5s} = \Gamma_{5v}^{(4)}$ denoted by $|\uparrow_h\rangle$, $|\downarrow_h\rangle$ (referred to as the doublet LH bands), respectively. Since both of the HH and LH bands belong to the same doublet irreps. $\Gamma_{5v}$, it is natural to consider $\Gamma'_{5v} = \Gamma_{5v}^{(2)} + \tilde{\beta}_{HL}\Gamma_{5v}^{(4)}$ for the valence hole states of QDs in the $C_{2v}$ symmetry, where the complex coefficient $\tilde{\beta}_{HL} \equiv \beta_{HL}e^{-i\phi_\beta}$ reflects the degree of valence band mixing (VBM) and is essentially determined by the symmetry of system. For a $C_{2v}$ QD, $\Gamma_{5v}^{(2)}$ and $\Gamma_{5v}^{(4)}$ keep invariant under the action of the symmetry transformations ($C_{2z}$, $\sigma_y$, $\sigma_x$,...) in Table S2 for $C_{2v}$ group, of course so do $\Gamma'_{5v}$. Carrying out a symmetry transformation might yield an additional phase angle to $\phi_\beta$. For example, a rotation $e^{i\theta}$ will add an angle $\theta$ to the phase angle $\phi'_\beta = \phi_\beta + \theta$. It can be shown that only certain phase angles, $\phi'_\beta$, can keep $\Gamma'_{5v}$ invariant under the symmetry transformations. With the arbitrary value of $\tilde{\beta}_{HL}$, the mixture of HH and LH, $\Gamma'_{5v} = \Gamma_{5v}^{(2)} + \tilde{\beta}_{HL}\Gamma_{5v}^{(4)}$, might not belong to a representation of $C_{2v}$ if the chosen phase angle $\phi'_\beta$ is improper to the symmetry of the system. For a $C_{2v}$ QD, only the phase angles, $\phi_\beta = 0$ or $\pi$, can match the symmetry, which indicates a real number of $\tilde{\beta}_{HL}$. The prediction of real $\beta_{HL}$ for a $C_{2v}$ QD is consistent with the analysis based on the real electronic structures of QDs as presented in the main article.

With the nature of VBM, the exciton states are created from the direct product of the $\Gamma_{5c}$ conduction band and the $\Gamma'_{5v}$ valence band coupled by the electron-hole Coulomb interaction, $\Gamma_{5c} \times \Gamma'_{5v} = \Gamma_{1X} + \Gamma_{2X} + \Gamma_{3X} + \Gamma_{4X}$, where $\Gamma_{2X}$ and $\Gamma_{4X}$ ($\Gamma_{1X}$ and $\Gamma_{3X}$) stand for the high-lying (low-lying) exciton states.

In the group $C_{2v}$, the irrep. for photon reduces to three singlet irreps. $\Gamma_5^{(T_d)} = \Gamma_1 + \Gamma_2 + \Gamma_4$, and the "vacuum state" with no exciton belongs to the singlet irrep. $\Gamma_1$. The direct products of the irreps. for photon and exciton are given by

$$\Gamma_1 \in \Gamma_1 \times \Gamma_{1X} = \Gamma_1, \tag{4}$$

$$\Gamma_1 \in \Gamma_2 \times \Gamma_{2X} = \Gamma_1, \tag{5}$$

$$\Gamma_1 \in \Gamma_4 \times \Gamma_{4X} = \Gamma_1, \tag{6}$$

$$\Gamma_1 \notin \Gamma_1/\Gamma_2/\Gamma_4 \times \Gamma_{3X} = \Gamma_3/\Gamma_4/\Gamma_2. \tag{7}$$

Accordingly, one can infer the existence of three BX states $\Gamma_{1X}$, $\Gamma_{2X}$ and $\Gamma_{4X}$ and that of DX singlet $\Gamma_{3X}$ according to the Wigner-Eckart theorem. Further, from the basis functions associated with the irreducible representation in Table S2, we are aware that the three BX

states, $\Gamma_{1X}$, $\Gamma_{2X}$ and $\Gamma_{4X}$ are optically polarized in the $z$-, $x$- and $y$- directions, respectively. In this work, we are mainly interested in the $x$- and $y$-polarized BX states ($\Gamma_{2X}$ and $\Gamma_{4X}$) that emit light vertically out of the QDs grown on the (001) substrate.

### C. QDs with tuning knobs

In principle, the four exciton states of a $C_{2v}$ QD that belong to the different irreducible representations should own distinctive energies. Thus, the only possibility of crossing over the energy levels of the $\Gamma_{2X}$ and $\Gamma_{4X}$ exciton states of a $C_{2v}$ QD is by means of accidental degeneracy that might be made by external tuning knobs. As pointed out by Singh and Bester in Ref.[1], such a level-crossing of the $\Gamma_{2X}$ and $\Gamma_{4X}$ BX states could happen only as the two BX states belong to *different* irrep. as shown in Table S2 for $C_{2v}$ QDs. Therefore, a full elimination of the FSS of a $C_{2v}$ QD by tuning knobs can be possible if the $C_{2v}$ symmetry of the QD can be surely preserved during the tuning process. In reality, imposing tuning knobs onto a QD yet likely breaks and reduces the $C_{2v}$ symmetry to lower ones, say $C_2$.

For a QD with the $C_2$ symmetry lowered by tuning knobs, the conduction band becomes the doublet irreps. $\Gamma_{3c}$ and so do the topmost valence band $\Gamma_{3v}$ due to the SOI. With the electron-hole Coulomb interactions, the four bright exciton states turn out to belong to $2\Gamma_{1X} + 2\Gamma_{2X}$ (See the character table of group $C_2$ in Table S3), among which the $x$- and $y$-polarized BX states which we are mainly interested in turn out to be in the same irrep. $\Gamma_{2X}$. If the symmetry of QD is lowered to be even lower, i.e. the $C_1$ symmetry, all the four excitons belong to the *same* irrep. $\Gamma_{1X}$ and become bright. Therefore, as long as the $C_{2v}$ symmetry of a QD is lowered by the application of tuning knobs to $C_2$ or even $C_1$, the two $x$- and $y$-polarized BX states become to belong to the same irreps. and it is no longer possible to eliminate the FSS of the QD. Thus, for the purpose of this work, one should seek for the useful stress actuators that can significantly tune the FSSs of QDs and still can preserve the $C_{2v}$ symmetry of the QDs.

TABLE S3: **The character table of group $C_2$.**

| $C_2$ | $E$ | $C_2$ | Basis function |
|---|---|---|---|
| $\Gamma_1$ | 1 | 1 | $z$ |
| $\Gamma_2$ | 1 | $-1$ | $x, y$ |
| $\Gamma_3$ | 2 | 0 | |

## S2. THE TENSOR OF STRAIN INDUCED BY AN IN-PLANE UNI-AXIAL STRESS

In this section, we present how to derive the tensor of strain induced by an in-plane uni-axial stress acting on a zinc-blende semiconductor quantum dot along an arbitrary in-plane direction. The derivation of the strain tensor consists of the following steps. First, we rotate the in-plane coordinate axes in the Cartesian reference frame, $Ox_1$ and $Ox_2$, to the new ones, $Ox_1'$ and $Ox_2'$, so that the new $Ox_1'$ axis is aligned to that of the uni-axial stress. In the new reference frame where the uni-axial stress is along the $x_1'$-axis, it is straightforward to have the explicit form of strain tensor. After we acquire the strain tensor in $Ox_1'x_2'x_3$, we re-rotate the reference frame back to $Ox_1x_2x_3$. at last, one can follow the formalism of tensor transformation in Ref. [2], to derive the strain tensor in the original reference frame $Ox_1x_2x_3$.

### A. Transformation of stress tensor under a rotation of coordinate axes

Regarding the rotation of the Cartesian reference frame counterclockwise around the $x_3$ axis by an angle $\phi$, the transformation matrix that relates the coordinates in the new reference frame, $(x_1', x_2', x_3')$, and those in the original one, $(x_1, x_2, x_3)$, reads [3]

$$[a_{ij}] = \begin{pmatrix} a_{11} & a_{12} & a_{13} \\ a_{21} & a_{22} & a_{23} \\ a_{31} & a_{32} & a_{33} \end{pmatrix} = \begin{pmatrix} \cos\phi & \sin\phi & 0 \\ -\sin\phi & \cos\phi & 0 \\ 0 & 0 & 1 \end{pmatrix}, \tag{8}$$

The coordinate transformation follows the equations given below,

$$x_i' = a_{ij} x_j \tag{9}$$

or

$$x_i = a_{ji} x'_j \,. \tag{10}$$

For brevity, hereby we adopt the Einstein notation for summation.

The transformations law for the tensor of the fourth rank, $T_{ijkl}$, such as elastic compliance- or stiffness-tensors, is given by [2]

$$T'_{ijkl} = a_{im} a_{jn} a_{ko} a_{lp} T_{mnop} \tag{11}$$

or

$$T_{ijkl} = a_{mi} a_{nj} a_{ok} a_{pl} T'_{mnop} \,. \tag{12}$$

Now, let us apply the transformation law to derive the tensor of an uni-axial stress of strength $\sigma$ rotated from the $x_1$ axis by an angle $\phi$, as depicted in Fig.S1. In the case, the stress tensor, $[\sigma'_{ij}]$, in the new reference frame is straightforwardly given by

$$\sigma'_{ij} = \begin{cases} \sigma, \text{ if } i = j = x'_1 \\ 0, \text{ else} \end{cases} \tag{13}$$

According to Eq.(11), the non-zero tensor elements of the uni-axial stress in the original reference frame is derived from $\sigma_{ij} = a_{ki} a_{lj} \sigma'_{kl}$ and given by

$$\begin{bmatrix} \sigma_{x_1x_1} \\ \sigma_{x_2x_2} \\ \sigma_{x_3x_3} \end{bmatrix} = \begin{bmatrix} \cos^2\phi & \sin^2\phi & -\sin 2\phi \\ \sin^2\phi & \cos^2\phi & \sin 2\phi \\ \frac{1}{2}\sin 2\phi & -\frac{1}{2}\sin 2\phi & \cos 2\phi \end{bmatrix} \begin{bmatrix} \sigma \\ 0 \\ 0 \end{bmatrix}' = \sigma \begin{bmatrix} \cos^2\phi \\ \sin^2\phi \\ \frac{1}{2}\sin 2\phi \end{bmatrix} \tag{14}$$

where the prime superscript on the column vector indicates the coordinate in the new frame reference frame.

### B. Transformation of strain tensor

We proceed with deriving the strain tensor from Eq.(14). As mentioned in the main text, it has been established that GaAs DE-QDs on (001) substrate are usually elongated along the axis $[1\bar{1}0]$. Thus, it is straightforward to adopt the reference frame where $\hat{x}'_1 || [1\bar{1}0] \equiv \hat{x}$, $\hat{x}'_2 || [110] \equiv \hat{y}$ and $\hat{x}'_3 || [001] \equiv \hat{z}$. As shown in Ref.[4], the relationship between the tensor of stress and that of the resultant strain represented in the reference frame for zinc-blende

GaAs is given by

$$\begin{bmatrix} \varepsilon_{xx} \\ \epsilon_{yy} \\ \epsilon_{zz} \\ 2\epsilon_{yz} \\ 2\epsilon_{xz} \\ 2\epsilon_{xy} \end{bmatrix} = \begin{bmatrix} s'_{11} & s'_{12} & s'_{13} & 0 & 0 & 0 \\ s'_{21} & s'_{22} & s'_{23} & 0 & 0 & 0 \\ s'_{31} & s'_{32} & s'_{33} & 0 & 0 & 0 \\ 0 & 0 & 0 & s'_{66} & 0 & 0 \\ 0 & 0 & 0 & 0 & s'_{66} & 0 \\ 0 & 0 & 0 & 0 & 0 & s'_{66} \end{bmatrix} \begin{bmatrix} \sigma_{xx} \\ \sigma_{yy} \\ \sigma_{zz} \\ \sigma_{yz} \\ \sigma_{xz} \\ \sigma_{xy} \end{bmatrix} \tag{15}$$

where

$$\begin{aligned} s'_{11} &= s'_{22} = \frac{1}{2}(s_{11}+s_{12}) + \frac{1}{4}s_{44} \\ s'_{12} &= s'_{21} = \frac{1}{2}(s_{11}+s_{12}) - \frac{1}{4}s_{44} \\ s'_{13} &= s'_{23} = s'_{31} = s'_{32} = s_{12} \\ s'_{33} &= s_{11} \\ s'_{66} &= 2(s_{11}-s_{12})\,, \end{aligned} \tag{16}$$

where $s_{11} = 0.0082\text{GPa}^{-1}$, $s_{12} = -0.002\text{GPa}^{-1}$, and $s_{44} = 0.0168\text{GPa}^{-1}$ are the elastic compliance constants for GaAs. [4, 5]

According to Eqs.(14) and (15), the strain tensor due to an in-plane uni-axial stress of magnitude $\sigma$ along the direction with a angle $\phi$ with respect to the elongation of QD, $[1\bar{1}0]$-axis, is given by

$$\begin{aligned} \epsilon_{xx} &= \frac{1}{2}(s_{11}+s_{12})\cdot\sigma + \frac{s_{44}}{4}(\sigma\cdot\cos 2\phi) \\ \epsilon_{yy} &= \frac{1}{2}(s_{11}+s_{12})\cdot\sigma - \frac{s_{44}}{4}(\sigma\cdot\cos 2\phi) \\ \epsilon_{xy} &= \frac{1}{2}(s_{11}-s_{12})\cdot(\sigma\cdot\sin 2\phi) \end{aligned} \tag{17}$$

$$\epsilon_{zz} = (s_{11}+s_{12})\cdot\sigma\,. \tag{18}$$

### C. The strain induced by $N$ in-plane uni-axial stresses

In the latest micro-electro-mechanical technology, a set of multiple separately tunable uni-axial stresses can be generated by micro-machined piezoelectric PMN-PT actuators, and

the resulting strain is transferred to QDs by bonding the QD membrane onto the PMN-PT crystal. According to Eq.(14), the total stress of $N$ uni-axial stresses is written as

$$\sum_i^N \boldsymbol{\sigma}_i = \sum_i^N \sigma_i \begin{bmatrix} \cos^2\phi_i \\ \sin^2\phi_i \\ \frac{1}{2}\sin 2\phi_i \end{bmatrix}, \tag{19}$$

where $i = 1, 2, ...N$ specifies the $i$-th uni-axial stress. By substituting Eq.(19) into Eq.(15), one can derive the resultant strain from the $N$ uni-axial stresses as

$$\epsilon_{xx} = \frac{s_{11}+s_{12}}{2}\cdot(\sum_{i=1}^N \sigma_i) + \frac{s_{44}}{4}\cdot(\sum_{i=1}^N \sigma_i \cos 2\phi_i) \tag{20}$$

$$\epsilon_{yy} = \frac{s_{11}+s_{12}}{2}\cdot(\sum_{i=1}^N \sigma_i) - \frac{s_{44}}{4}\cdot(\sum_{i=1}^N \sigma_i \cos 2\phi_i) \tag{21}$$

$$\epsilon_{xy} = \frac{s_{11}-s_{12}}{2}\cdot(\sum_{i=1}^N \sigma_i \sin 2\phi_i) \tag{22}$$

$$\epsilon_{zz} = (s_{11}+s_{12})\cdot(\sum_{i=1}^N \sigma_i)\,. \tag{23}$$

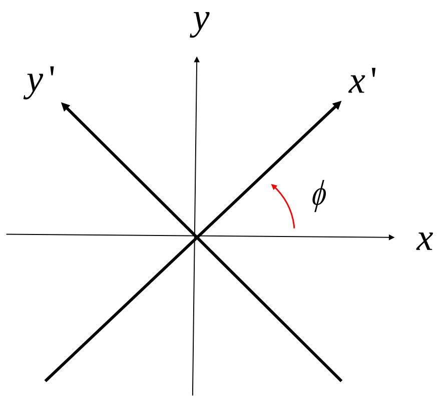


FIG. S1: Schematic of rotated coordinate systems.

### D. The strain generated by dual uni-axial stresses in the $C_{2v}$ symmetry

The $C_{2v}$ point group consists of the operations, $E$, $C_2$, $\sigma_x$, and $\sigma_y$, whose representations in matrix are, respectively, given by

$$E = \begin{bmatrix} 1 & 0 & 0 \\ 0 & 1 & 0 \\ 0 & 0 & 1 \end{bmatrix}, \tag{24}$$

$$C_2 = \begin{bmatrix} -1 & 0 & 0 \\ 0 & -1 & 0 \\ 0 & 0 & 1 \end{bmatrix}, \tag{25}$$

$$\sigma_y = \begin{bmatrix} 1 & 0 & 0 \\ 0 & -1 & 0 \\ 0 & 0 & 1 \end{bmatrix}, \tag{26}$$

$$\sigma_x = \begin{bmatrix} -1 & 0 & 0 \\ 0 & 1 & 0 \\ 0 & 0 & 1 \end{bmatrix}. \tag{27}$$

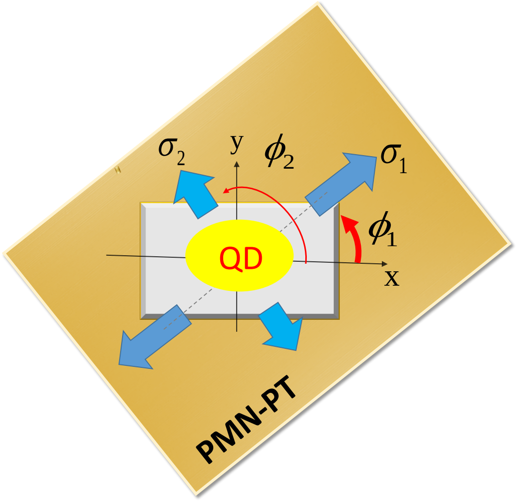


FIG. S2: Schematic top view of a GaAs/AlGaAs QD under a set of two uni-axial stresses ($\sigma_1$ and $\sigma_2$) from a PMN-PT actuator.

If the symmetry of a $C_{2v}$ QD is not affected by a set of externally applied stresses, the resulting strain tensor from the stress should be in the $C_{2v}$ symmetry as well. According to Neumann's principle, the resulting strain tensor from the stress must be kept invariant under any operations in the $C_{2v}$ point group, i.e.

$$\epsilon'_{ij} = \epsilon_{ij} \ , \tag{28}$$

where $\epsilon'_{ij} = a_{il}a_{jm}\epsilon_{lm}$ and $[a_{ij}] = E, C_{2v}, \sigma_x, \sigma_y$. Accordingly, one can show that the strain tensor fulfilling the $C_{2v}$ symmetry must be in the form where $\epsilon_{ij} = 0$ if $i \neq j$. From Eq.(22), one can show that $\epsilon_{ij} = 0$ for $i \neq j$ if and only if

$$\sum_{i=1}^{N} \sigma_i \sin 2\phi_i \tag{29}$$

In other words, if a set of $N$ in-plane uni-axial stresses satisfy Eq.(29), their resulting strain is surely in the $C_{2v}$ symmetry.

## S3. MODEL ANALYSIS FOR THE FINE STRUCTURES OF QDS

For analysis, we might treat the couplings between heavy-hole (HH) and light-hole (LH) components as a perturbation to the VBM exciton states of QDs as conducted in previous studies Refs.[7, 8], and write the excite doublet as $|\downarrow_e\Uparrow'_h\rangle \approx |\downarrow_e\Uparrow_h\rangle - \tilde{\beta}^*_{HL}|\downarrow_e\downarrow_h\rangle$ ($|\uparrow_e\Downarrow'_h\rangle \approx |\uparrow_e\Downarrow_h\rangle - \tilde{\beta}_{HL}|\uparrow_e\uparrow_h\rangle$), where $\tilde{\beta}_{HL}$ are the coefficients of the leading LH components in the exciton states.

The envelop wave functions of the leading HH and LH components are modelled in the parabolic model by $\langle\vec{r}|\Uparrow_h / \Downarrow_h\rangle \approx \phi_0(\vec{r})u_{j_z=+/-\frac{3}{2}}(\vec{r})$ and $\langle\vec{r}|\uparrow_h / \downarrow_h\rangle \approx \phi_0(\vec{r})u_{j_z=+/-\frac{1}{2}}(\vec{r})$, where $\phi_0(\vec{r}) = \sqrt{\frac{1}{\pi^{3/2}l_x l_y l_z}} \exp\left\{-\frac{1}{2}\left[\left(\frac{x}{l_x}\right)^2 + \left(\frac{y}{l_y}\right)^2 + \left(\frac{z}{l_z}\right)^2\right]\right\}$ is the wave function of the lowest Fock-Darwin state in the parabolic model and $l_{\alpha=x,y,z}$ is the characteristic length of the wave function extent along the $\alpha$-direction. Accordingly, the coefficient of the leading LH component is formulated as [4, 7]

$$\widetilde{\beta}_{HL} \approx \frac{\rho_{HL}}{\Delta_{HL}} \tag{30}$$

where $\rho_{HL} = \langle\phi_0|R_k + R_\epsilon|\phi_0\rangle = \langle\phi_0|R_k|\phi_0\rangle + \langle\phi_0|R_\epsilon|\phi_0\rangle$, $\rho^0_{HL} + \rho^\epsilon_{HL}$
$\Delta_{HL} = \langle\phi_0|P - Q|\phi_0\rangle - \langle\phi_0|P + Q|\phi_0\rangle = -2\langle\phi_0|Q_k|\phi_0\rangle - 2\langle\phi_0|Q_\epsilon|\phi_0\rangle = \Delta^0_{HL} + \Delta^\epsilon_{HL}$.

In the approximation, one can derive a simplified effective Hamiltonian for the VBM exciton doublet of a QD as presented in Ref.[8]. We shall show that our derived effective exciton Hamiltonian from the multi-band theory is consistent with and, with the proper inclusion of LH components, even beyond the model Hamiltonian given by Gong *et al.* in Ref.[10]. In the latter, only linear stress terms are assumed and preserved in the Hamiltonian. Thus, the model Hamiltonian in Ref.[10] is suited for the QDs with large HH-LH energy level separation, such as inherently strained InAs QDs. For unstrained GaAs DE-QDs with smaller HH-LH energy level, the valence-band-mixing (VBM) effects turn out to be more pronounced and the model Hamiltonian, however, does not fully capture the effects from other types of stress, such as bi-axial stress, which is essentially associated with the underlying VBM in the exciton states.

For comparison with the model Hamiltonian in Ref.[10], we adopt the same exciton basis defined by $\frac{1}{\sqrt{2}}(|\downarrow_e \Uparrow'_h\rangle \pm |\uparrow_e \Downarrow'_h\rangle)$, in which the effective exciton Hamiltonian reads

$$H'_X = \begin{pmatrix} E_X^{(0)} + \Re[\tilde{\Delta}_{eff}] & \Im[\tilde{\Delta}_{eff}] \\ -\Im[\tilde{\Delta}_{eff}] & E_X^{(0)} - \Re[\tilde{\Delta}_{eff}] \end{pmatrix} . \tag{31}$$

In the model, the *e-h* exchange interaction between the BX doublet can be formulated as

$$\widetilde{\Delta}_{eff} = -\Delta_1 + \frac{2}{\sqrt{3}} E_X^S \cdot \widetilde{\beta}_{HL} \tag{32}$$

where $\Delta_1$ is the matrix element of the long-ranged e-h exchange interaction involving only the HH-component of the hole state, the second term on the RHS is the short-ranged e-h exchange interaction arising from VBM reflected by $\widetilde{\beta}_{HL} = \beta_{HL} e^{-i\theta_\beta}$ , $E_X^S$ as an empirical parameter is given by the *e-h* exchange splitting between the BX and DX states in GaAs bulk by extrapolation. Note that $\Delta_1$ is stress-insensitive while $\tilde{\Delta}_{VBM}$ is associated with VBM and highly tunable by external stress.

For GaAs DE-QDs with two uni-axial stresses, by taking the fact that $l_x, l_y \gg l_z$ and $\frac{d}{4} s_{44} \approx \frac{\sqrt{3}}{2} b(s_{11} - s_{12})$, one derives $\rho^{\epsilon}_{HL} \approx \lambda(\sigma_1 e^{2i\phi_1} - \sigma_2 e^{2i\phi_2})$, $\Delta^{\epsilon}_{HL} = -\frac{b}{2}(s_{11} - s_{12})(\sigma_1 + \sigma_2) = \mu(\sigma_1 + \sigma_2)$ and

$$\widetilde{\beta}_{HL} = \frac{\rho^0_{HL} + \lambda(\sigma_1 e^{2i\phi_1} - \sigma_2 e^{2i\phi_2})}{\Delta^0_{HL} + \mu(\sigma_1 + \sigma_2)} , \tag{33}$$

where $\lambda \equiv \frac{d}{4} s_{44}$, $\mu \equiv -\frac{b}{2}(s_{11} - s_{12})$, $\rho^0_{HL} = \frac{\sqrt{3}\hbar^2\gamma_3}{4m_0}\left(\frac{1}{l_y^2} - \frac{1}{l_x^2}\right)$, $\Delta^0_{HL} \approx \frac{\hbar^2\gamma_2}{m_0}\frac{1}{l_z^2}$. Equation (33) shows the stress-tunability of VBM, making the e-h exchange interaction in Eq.(32) stress-tunable as well.

According to Eq.(32), The fine structure splitting of exciton is given by

$$S = 2\sqrt{(\Im[\tilde{\Delta}_{eff}])^2 + (\Im[\tilde{\Delta}_{eff}])^2} \tag{34}$$
$$= 2\sqrt{(\Im[\tilde{\Delta}_{VBM}])^2 + (-\Delta_1 + \Re[\tilde{\Delta}_{VBM}])^2}\,,$$

where $\tilde{\Delta}_{VBM} \equiv \frac{2}{\sqrt{3}} E_X^S \cdot \widetilde{\beta}_{HL}$. Equation (35) shows that $S = 0$ requires that the both of real and imaginary parts of the exchange interaction vanish, i.e. $\Im[\tilde{\Delta}_{eff}] = 0$ and $\Re[\tilde{\Delta}_{eff}] = 0$. The former condition is equivalent that $\Im[\tilde{\Delta}_{VBM}] = 0$, i.e. $\Im[\tilde{\beta}_{HL}] = 0$, which, from Eq.(33), leads to $\sigma_1 \sin 2\phi_1^\sigma + \sigma_2 \sin 2\phi_2^\sigma = 0$, as derived by the group theory presented in the main text.

As one can preserve $\Im[\tilde{\Delta}_{VBM}] = 0$ during the tuning of $S$, one might further adjust $\Re[\tilde{\Delta}_{VBM}]$ to cancel out $\Delta_1$ so as to achieve $S = 0$. Hence, in usual cases, two tuning knobs are needed for certain elimination of $S$. As one of our main findings in the work, it is shown that one needs only one tuning knob to make $S = 0$ as long as the knob can tune $\Re[\tilde{\beta}_{HL}]$ and simultaneously keep $\Im[\tilde{\beta}_{HL}] = 0$. Symmetric bi-axial is an example in the case. As presented in the main text, a symmetric bi-axial stress generates the strain that always preserves $\Im[\tilde{\beta}_{HL}] = 0$ (substituting $\sigma_1 = \sigma_2$ and $\phi_1 = \phi_2 - 90°$ in Eq.(33)) and can be used to tune $\Re[\tilde{\beta}_{HL}]$ (because of the bi-axial stress term in the denominator of Eq.(33)). In fact, a symmetric bi-axial can substantially affect VBM and the resultant *e-h* exchange interaction but does not reduce the original $C_{2v}$ symmetry of elongated QDs.

The theory comprised of Eqs.(31)-(35) is consistent with and even more general than the existing exciton model established by Gong *et al.* in Ref.[10]. It is straightforward to reproduce the model Hamiltonian in Ref.[10] by removing bi-axial term in the denominator of Eq.(33). Ignoring the bi-axial term and setting $\sigma_2 = 0$, the Hamiltonian in Eq.(31) turns out to be in the same form as Ref.[10],

$$H_X'' = \begin{pmatrix} E + \delta + \alpha_3 p & \beta p \\ \beta p & E - \delta + \alpha_4 p \end{pmatrix} \tag{35}$$

, which can be connected to our model via the following equations

$$p = \sigma_1 \tag{36}$$

$$\beta = k\frac{\lambda \sin 2\phi_1}{\Delta^0_{HL}} \tag{37}$$

$$\delta = -\Delta_1 + k\frac{\rho^0_{HL}}{\Delta^0_{HL}} \tag{38}$$

$$\alpha_3 = \frac{\lambda \cos 2\phi_1}{\Delta^0_{HL}} \tag{39}$$

$$\alpha_4 = -\frac{\lambda \cos 2\phi_1}{\Delta^0_{HL}}\ . \tag{40}$$

The neglect of the bi-axial term is acceptable as $\Delta^0_{HL} \gg \mu(\sigma_1 + \sigma_2)$, i.e. that the energy separation of the HH- and LH-level is much greater than the deformation potential of the applied bi-axial stress. This is suited for the case of inherently strained InGaAs/AlGaAs SK-QDs, but not for un-strained GaAs/AlGaAs DE-QDs. For InGaAs/AlGaAs SK-QDs, the HH and LH level energies are greatly separated by the inherent compressive bi-axial strain caused by the lattice mismatch between InGaAs and AlGaAs, and the application of external bi-axial stress that is typically 1-2 orders of magnitude smaller than the intrinsic stress in the QS, make only a limited influence on the excitonic fine structures. For GaAs/AlGaAs QDs, the absence of intrinsic strain brings the LH level closer to the HH ones in energy, and the effect of external bi-axial stress should not be neglected.

---


[1] R. Singh and G. Bester, Phys. Rev. Lett. **104**, 196803 (2010).

[2] J. F. Nye, *Physical Properties of Crystals*, Clarendon Press (1960).

[3] H. J. Weber, G. B. Arfken, *Essential Mathematical Methods for Physicists*, Elsevier Academic Press.

[4] S. Kumar, E. Zallo, Y. H. Liao, P. Y. Lin, R. Trotta, P. Atkinson, J. D. Plumhof, F. Ding, B. D. Gerardot, S. J. Cheng, A. Rastelli, and O. G. Schmidt, Phys. Rev. B **89**, 115309 (2014).

[5] S. L. Chuang, *Physics of Photonic Devices*, 2nd ed. John Wiley and Sons Ltd (2009).

[6] T. Takagahara, Phys. Rev. B **62**, 16840 (2000).

[7] Y. H. Liao, C. C. Liao, C. H. Ku, Y. C. Chang, and S. J. Cheng, M. Jo, T. Kuroda, T. Mano, M. Abbarchi, and K. Sakoda, Phys. Rev. B **86**,115323 (2012).

[8] S. J. Cheng, Y. H. Liao, and P. Y. Lin, Phys. Rev. B **91**, 115310 (2015).

[9] E. Kadantsev and P. Hawrylak, Phys. Rev. B **81**, 045311 (2010).

[10] M. Gong, W. Zhang, G.-C. Guo, and L. He, Phys. Rev. Lett. **106**, 227401 (2011).

[11] Y. N. Wu, M. F. Wu, Y. W. Ou, Y. L. Chou, and S. J. Cheng, Phys. Rev. B **96**, 085309 (2017)
